# Supplementary material for: Inferring Spatial Uncertainty in Object Detection
Source: arXiv:2003.03644 source file (2020-08-01)
Supplement: Supplementary file 1 [file appendix.tex]

\appendix
\subsection{Proof of Spatial Distribution}
This section give the equality of Eq.~\ref{eq:JIoU_def} based on the relationship between $v$ and $y$ given in Eq.~\ref{eq:zy_render}. 
\begin{proof}
From Eq.~\ref{eq:zy_render} and by denoting $Y=[C_1,C_2,C_3,L,W,H,r_Y]^T$, $C{:=}[C_1,C_2,C_3]^T$, $S{:=}[L,W,H]$ $R_Y$ as the rotation matrix of $r_Y$ and $v_0{:=}[v_1,v_2,v_3]^T$, we have
\begin{equation}
     R_Y^T(V{-}C)=\left[\begin{smallmatrix}l\\w\\h\end{smallmatrix}\right]\circ v_0,
\end{equation}
where $\circ$ denotes the element-wise multiplication (Hadmard product) of matrices. This equation means when conditioned on $r_Y{=}r_y$ and $C=[c_1,c_2,c_3]$, the mapping between $V$ and $S$ is a diffeomorphism and the probability density function of $V|r_Y,C$ is
\begin{equation}
    p_{V|r_y,c}(u) = \left|\frac{1}{v_1v_2v_3}\right|p_{S|r_y,c}\left
    (R_y^T(u{-}c)\circ v_0^{-1}\right),
\end{equation}
where $v_0^{-1}$ is the element-wise inverse of $v_0$. Then
\begin{equation}
    \begin{aligned}
    &\quad\ \int_{v_0\in B(y^*)}p_{V}\left(u\right)dv_0 \\
    &=\int_{v_0\in B(y^*)}\left(\int{p_{V|r_y,c}(u)}p_{r_Y,C}(r_y,c)dr_ydc\right)dv_0\\
    &=\int{p_{r_Y,C}dr_ydc\int_{v_0\in B(y^*)}{\left|\frac{1}{v_1v_2v_3}\right|p_{S|r_y,c}\left
    (R_y^T(u{-}c)\circ v_0^{-1}\right)dv_0}}\\
    &=\int{p_{r_Y,C}dr_ydc \int_{\{s|u\in B(c,s,r_y)\}}{\left|\frac{1}{l w h}\right|p_{S|r_y,c}\left
    (s\right)dldwdh}}\\
    &=\int_{\{c,s,r_y|u\in B(y),y=[c,s,r_y]\}}{\left|\frac{1}{l w h}\right|p_Y(c,s,r_y)dc ds dr_y}
    \end{aligned}.
\end{equation}
where $s{=}[l,w,h]^T$ are the length, width and height of the bounding box. Note that $\|lwh\|=A(y)$, hence Eq.~\ref{eq:JIoU_def} is proved.
\end{proof}

\subsection{How to Calculate Spatial Distribution}
The distribution $p_{V(v_0,Y)}(u)$ of $V(v_0,Y)$ is approximated by Gaussian distribution to reduce the computational load. Several possible situations may occur when calculating the spatial distribution defined by Eq.~\ref{eq:JIoU_def}:
\begin{enumerate}
    \item The distributions of some points of $V(v_0,Y)$, such as corners of the bounding box~\cite{hall2018probabilistic,meyer2019lasernet}, are predicted.
    \item The distribution of $Y$ is predicted but the distribution of $V$ is unknown, which are the cases of~\cite{feng2018leveraging,wirges2019capturing} and Section~\ref{sec:uncertainty}
\end{enumerate}

The moments of $V(v_0,Y)$ is related to $Y$ by Eq.~\ref{eq:zy_render}. Remember that Eq.~\ref{eq:zy_render} can be rewritten in the homogeneous coordinate of $v_0$ as
\begin{equation}
    v(v_0,y)=\Phi(y)^Tw,
\end{equation}
where $w$ is the homogeneous coordinate of $v_0$ and 
\begin{equation}
    \Phi(y)^T=\begin{bmatrix}
                l\cos(r_y) & 0 & -w\sin(r_y) & c_1\\
                0 & h & 0 & c_2\\
                l\sin(r_y)& 0 & w\cos(r_y) & c_3
                \end{bmatrix},
\end{equation}
is the feature matrix. Considering the assumption that we approximate the distribution of $V(v_0,Y)$ as Gaussian, we only need to calculate 
\begin{equation}
    \begin{aligned}
    E[V] &= E[\Phi(Y)]^Tw\\
    E[V^2] &= E[\Phi(Y)^Tww^T\Phi(Y)],
    \end{aligned}
\end{equation}
for all $w$'s corresponding to the points $v_0$ in the unit bounding box. For 3D, $ww^T\in \mathbb{R}^4$ is a symmetric matrix. Since the base of the set $Sym_4\left(\mathbb{R}\right)$ of symmetric matrices is 10, at most 10 points is enough for representing all possible $ww^T$'s. This means there exist a set $w_1,w_2,\cdots, w_{10}$ such that for any homogeneous coordinate $w$, there exist coefficients $\alpha_1, \alpha_2, \cdots, \alpha_{10}$ such that
\begin{equation}
    \sum_{i=1}^{10}{\alpha_i w_iw_i^T} = ww^T.
\end{equation}

Note that $w$ is homogeneous coordinate which means the 4th colum of $ww^T$ is $w$, so there is also
\begin{equation}
    \sum_{i=1}^{10}{\alpha_i w_i} = w.
\end{equation}

When we want to recover the uncertainty of parameters, specific $w$'s can be chosen. For the center $(c_1,c_2,c_3)$, choose $w_c=[0,0,0,1]^T$, so that
\begin{equation}
    E[\Phi(Y)w_cw_c^T\Phi(Y)]=E\left[\begin{bmatrix}
                c_1^2 & 0 & 0\\
                0 & c_2^2 & 0\\
                0& 0 & c_3^2
                \end{bmatrix}\right],
\end{equation}
gives the variance of the center parameters. For the length $l$, choose $w_l=[1,0,0,0]^T$, so that
\begin{equation}
\begin{aligned}
    E[l^2] &= trace\left(E[\Phi(Y)w_lw_l^T\Phi(Y)]\right)\\
    &=trace\left(E\left[\begin{bmatrix}
                l^2\cos^2(r_y) & 0 & 0\\
                0 & 0 & 0\\
                0& 0 & l^2\sin^2(r_y)
                \end{bmatrix}\right]\right),
\end{aligned}
\end{equation}

and for the width $w$, choose $w_w=[0,0,1,0]^T$ so that
\begin{equation}
\begin{aligned}
    E[w^2] &= trace\left(E[\Phi(Y)w_ww_w^T\Phi(Y)]\right)\\
    &=trace\left(E\left[\begin{bmatrix}
                w^2\sin^2(r_y) & 0 & 0\\
                0 & 0 & 0\\
                0& 0 & w^2\cos^2(r_y)
                \end{bmatrix}\right]\right),
\end{aligned}
\end{equation}
and for the height $h$, choose $w_h=[0,1,0,0]^T$ so that
\begin{equation}
\begin{aligned}
    E[h^2] &= trace\left(E[\Phi(Y)w_hw_h^T\Phi(Y)]\right)\\
    &=trace\left(E\left[\begin{bmatrix}
                0 & 0 & 0\\
                0 & h^2 & 0\\
                0& 0 & 0
                \end{bmatrix}\right]\right),
\end{aligned}
\end{equation}
